# Supplementary material for: Chameleon: Foundation Models for Fairness-aware Multi-modal Data Augmentation to Enhance Coverage of Minorities
Source: arXiv:2402.01071 source file (2024-02-02)
Supplement: Supplementary file 1 [file appendix.tex]

\section{Appendix}

\subsection{Subset Information}\label{sec:app:subsetinfo}
\begin{table}[!htbp]
  \centering
  \caption{\utkface Subset Counts by Combination}
  \label{tab:dataset1-counts}
  \begin{tabular}{@{}llrl@{}}
    \toprule
    \multicolumn{3}{c}{\textbf{Combination}} & \textbf{Count} \\
    \cmidrule(r){1-3} \cmidrule(l){4-4}
    \textbf{Race} & \textbf{Gender} & \textbf{Age-Group} & \\
    \midrule
    White & Male & Infant & 10 \\
    White & Male & Adult & 15 \\
    Black & Male & Infant & 8 \\
    % Add more rows for other combinations
    \bottomrule
  \end{tabular}
\end{table}

\begin{table}[htbp]
  \centering
  \caption{\feretdb Subset Counts by Combination}
  \label{tab:dataset2-counts}
  \begin{tabular}{@{}llr@{}}
    \toprule
    \multicolumn{2}{c}{\textbf{Combination}} & \textbf{Count} \\
    \cmidrule(r){1-2} \cmidrule(l){3-3}
    \textbf{Race} & \textbf{Gender} & \\
    \midrule
    White & Male & 20 \\
    White & Female & 25 \\
    Black & Male & 15 \\
    % Add more rows for other combinations
    \bottomrule
  \end{tabular}
\end{table}
